# Supplementary material for: Split-Treatment Analysis to Rank Heterogeneous Causal Effects for Prospective Interventions
Source: arXiv:2011.05877 source file (2020-11-11)
Supplement: Supplementary file 1 [file appendix.tex]

\clearpage
\begin{table*}
\caption{ Derivation of split treatment}
\centering
\begin{minipage}{0.75\textwidth}
\begin{align*}
    \text{ITE}(\bm{x}) = & \mathbb{E}[Y^{(z=1)}\mid \bm{x}] - \mathbb{E}[Y^{(z=0)}\mid \bm{x}] \\
    = & \mathbb{E}[Y\mid Z= 1, \bm{x}] - \mathbb{E}[Y \mid Z =0, \bm{x}]\\
    = & \mathbb{E}[Y\mid Z= 1, A= 1, \bm{x}]P(A=1|Z=1,\bm{x})P(Z=1|\bm{x}) + \mathbb{E}[Y\mid Z= 1, A= 0, \bm{x}]P(A=0|Z=1,\bm{x})P(Z=1|\bm{x}) \\
    & - \mathbb{E}[Y \mid Z =0, A=1, \bm{x}]P(A=1|Z=0,\bm{x})P(Z=0|\bm{x}) - \mathbb{E}[Y\mid Z= 0, A= 0, \bm{x}]P(A=0|Z=0,\bm{x})P(Z=0|\bm{x})\\
    = & \mathbb{E}[Y\mid A= 1, \bm{x}]P(A=1|Z=1,\bm{x})\cdot 1/2 + \mathbb{E}[Y\mid A= 0, \bm{x}]P(A=0|Z=1,\bm{x})\cdot 1/2\\
     & - \mathbb{E}[Y \mid A=1, \bm{x}]P(A=1|Z=0,\bm{x})\cdot 1/2 - \mathbb{E}[Y\mid A= 0, \bm{x}]P(A=0|Z=0,\bm{x})\cdot 1/2\\
    \propto & \mathbb{E}[Y\mid A= 1, \bm{x}]P(A=1|Z=1,\bm{x}) + \mathbb{E}[Y\mid A= 0, \bm{x}](1-P(A=1|Z=1,\bm{x}))\\ 
     & - \mathbb{E}[Y \mid A=1, \bm{x}]P(A=1|Z=0,\bm{x}) - \mathbb{E}[Y\mid A= 0, \bm{x}](1-P(A=1|Z=0,\bm{x}))\\
    = & (\mathbb{E}[Y\mid A= 1,\bm{x}] - \mathbb{E}[Y\mid A= 0, \bm{x}])P(A=1|Z=1,\bm{x}) + \mathbb{E}[Y\mid A= 0, \bm{x}]\\
    & - (\mathbb{E}[Y \mid A=1, \bm{x}]- \mathbb{E}[Y\mid A= 0, \bm{x}])P(A=1|Z=0,\bm{x}) - \mathbb{E}[Y\mid A= 0, \bm{x}]\\
    = & (\mathbb{E}[Y \mid A=1, \bm{x}]- \mathbb{E}[Y\mid A= 0, \bm{x}])(P(A=1|Z=1,\bm{x})- P(A=1|Z=0,\bm{x})) \\
    = & (\mathbb{E}[Y^{(a=1)} \mid \bm{x}]- \mathbb{E}[Y^{(a=0)}\mid \bm{x}])(P(A=1|Z=1,\bm{x})- P(A=1|Z=0,\bm{x}))
\end{align*}
\medskip
\hrule
\end{minipage}
\label{tab:dev}
\end{table*}

\begin{table*}
\caption{\divyat{I think the terms $P(Z=1|\bm{x})$ and $P(Z=0|\bm{x})$ shouldn't be there; see the justification below }}
\centering
\begin{minipage}{0.75\textwidth}
\begin{align*}
    \mathbb{E}[Y\mid Z= 1, \bm{x}] \\
    = & \int y*P(Y=y \mid Z=1, \bm{x}) \,dy \\
    = & \int y*\Big[ P(Y=y, A=1 \mid Z=1, \bm{x}) + P(Y=y, A=0 \mid Z=1, \bm{x}) \Big] \,dy \\
    = & \int y*\Big[ P(Y=y \mid A=1, Z=1, \bm{x})*P(A=1 \mid Z=1, \bm{x}) + P(Y=y \mid A=0, Z=1, \bm{X})*P(A=0 \mid Z=1, \bm{x}) \Big] \,dy \\  
    = & \Big( \int y*[ P(Y=y \mid A=1, Z=1, \bm{x})] \,dy \Big)*P(A=1 \mid Z=1, \bm{x}) + \Big( \int y*[ P(Y=y \mid A=0, Z=1, \bm{X}) ] \,dy \Big)*P(A=0 \mid Z=1, \bm{x}) \\  
    = & \mathbb{E}[Y\mid Z=1, A=1, \bm{x}]*P(A=1 \mid Z=1, \bm{x}) + \mathbb{E}[Y\mid Z=1, A=0, \bm{x}]*P(A=0 \mid Z=1, \bm{x})  
\end{align*}
\medskip
\hrule
\end{minipage}
\label{tab:dev}
\end{table*}

% \begin{lstlisting}
% // Hello.java
% import javax.swing.JApplet;
% import java.awt.Graphics;

% public class Hello extends JApplet {
%     public void paintComponent(Graphics g) {
%         g.drawString("Hello, world!", 65, 95);
%     }    
% }
% \end{lstlisting}

% \begin{figure*}
%     \centering
%     \includegraphics[width= \textwidth]{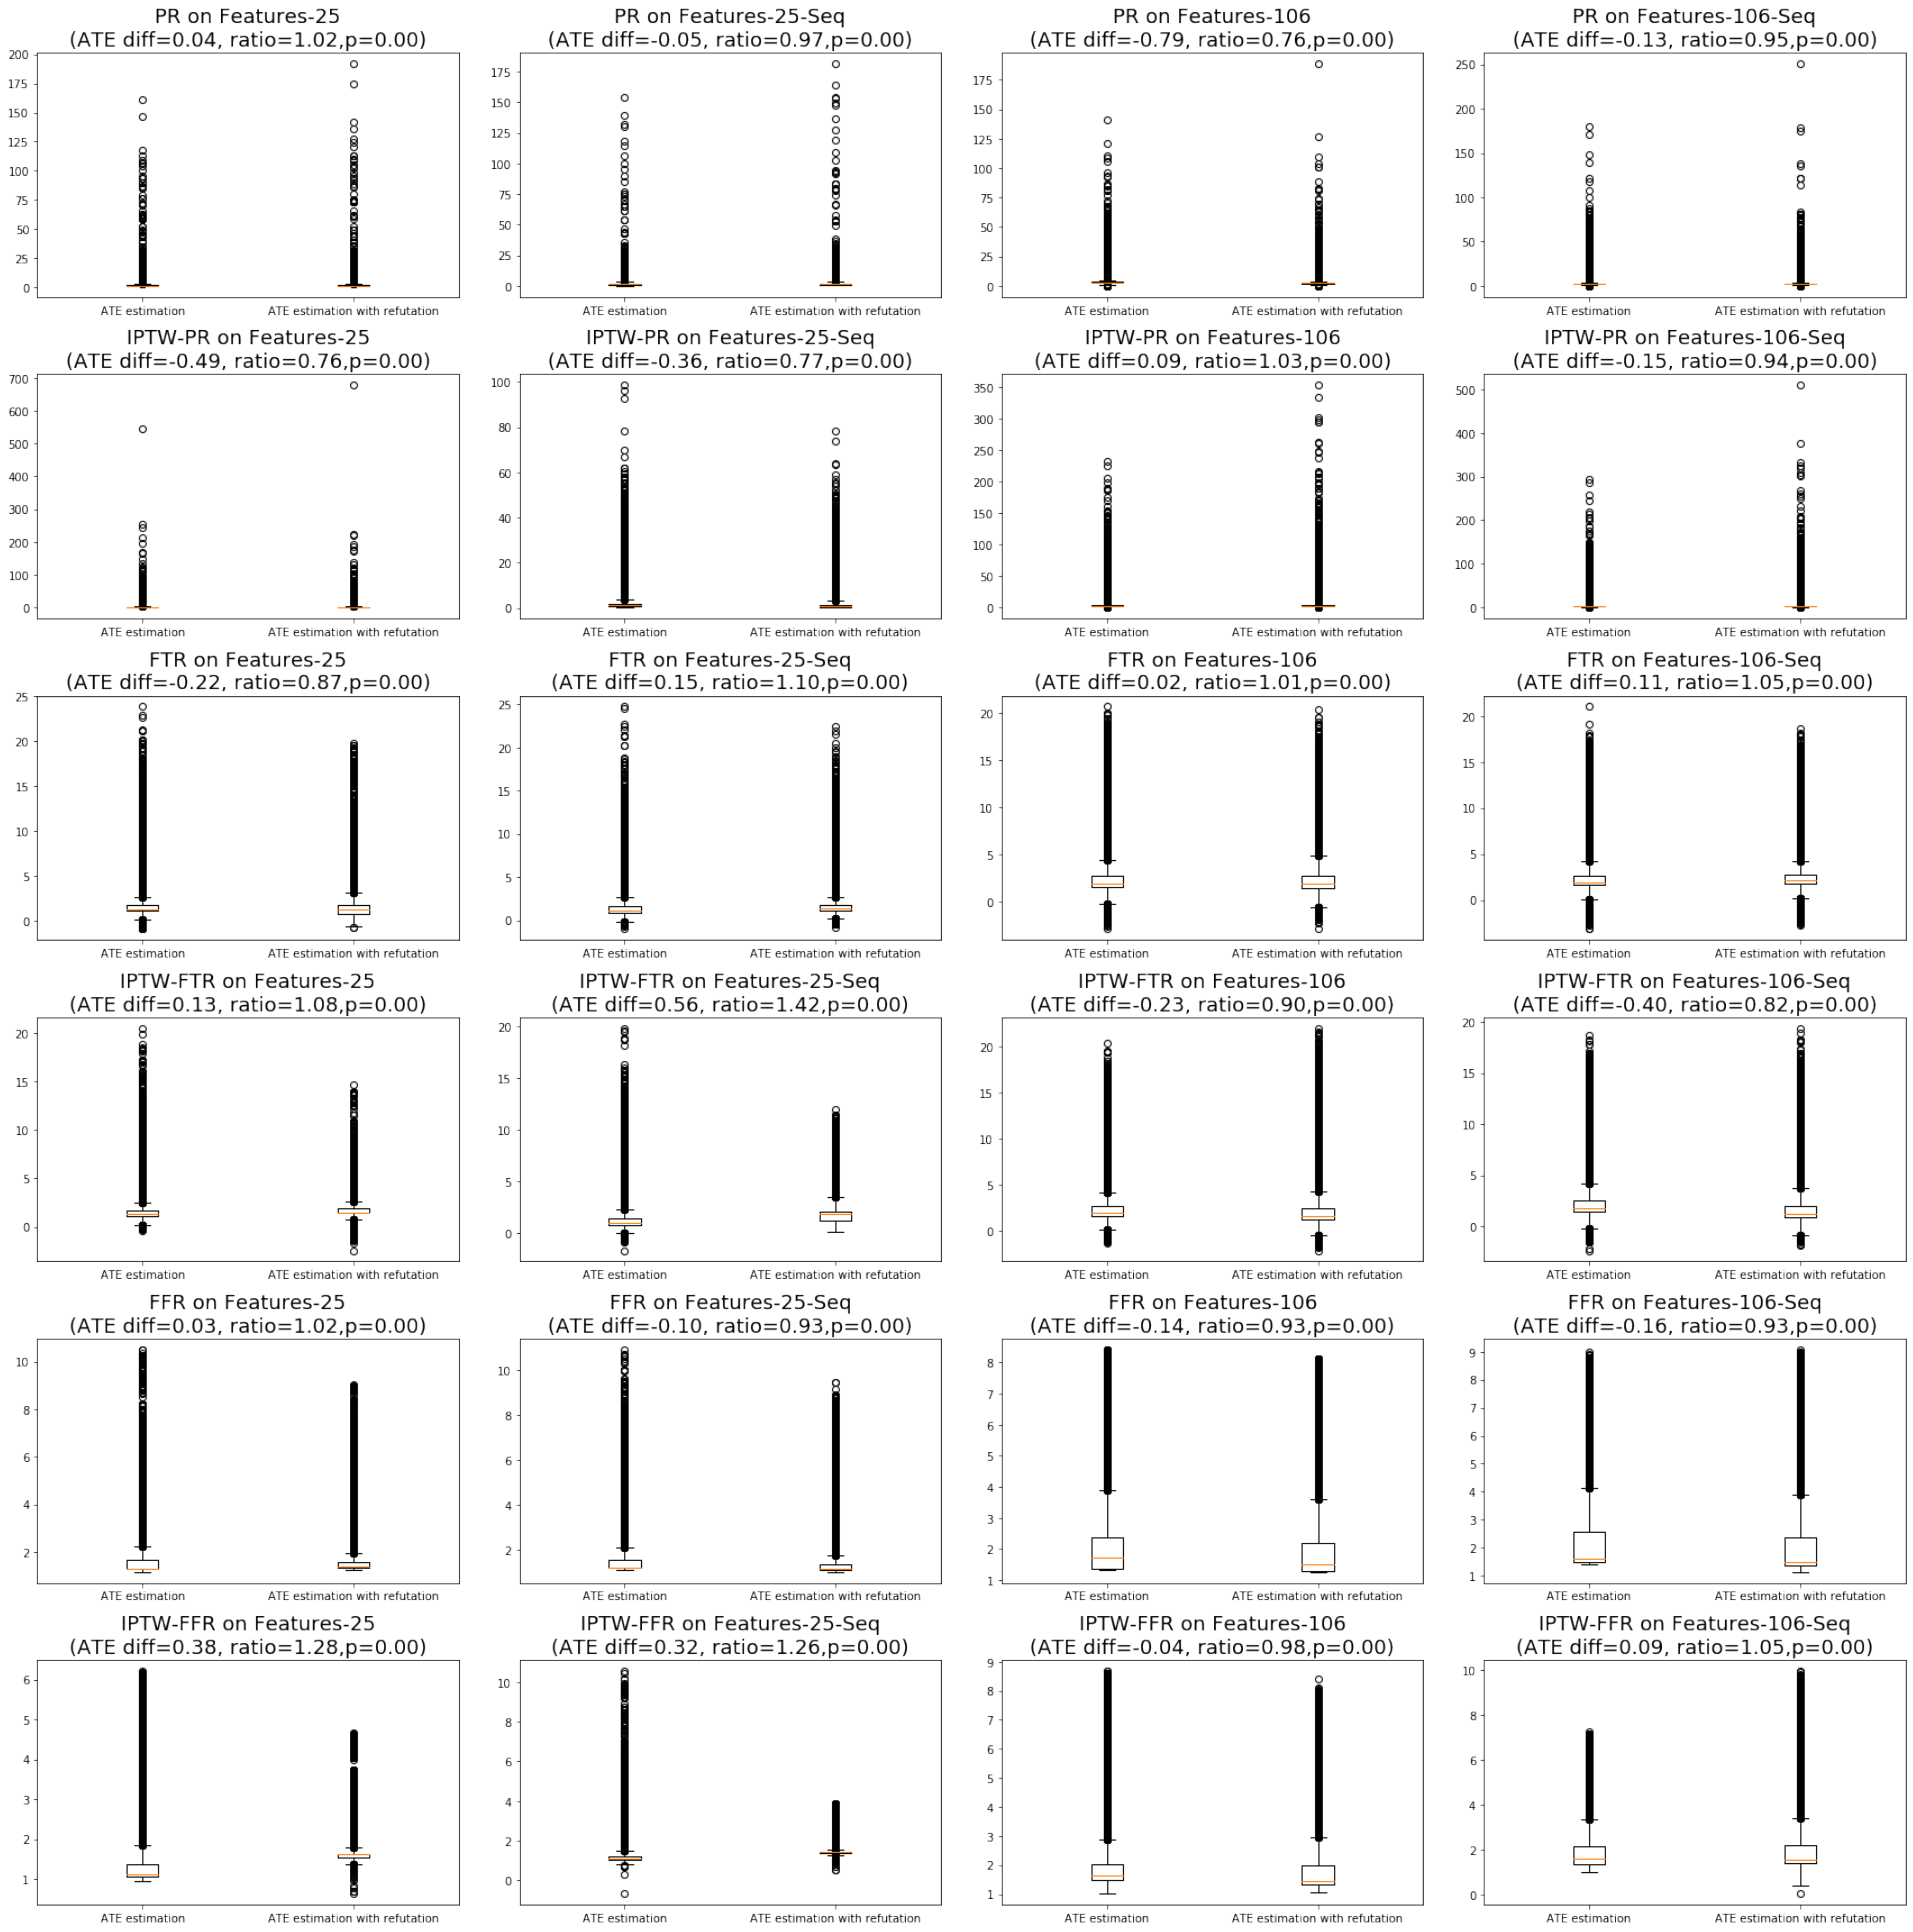}
%     \caption{Sensitivity analysis}
% \end{figure*}

% \begin{figure*}
%     \centering
%     \includegraphics[width= \textwidth]{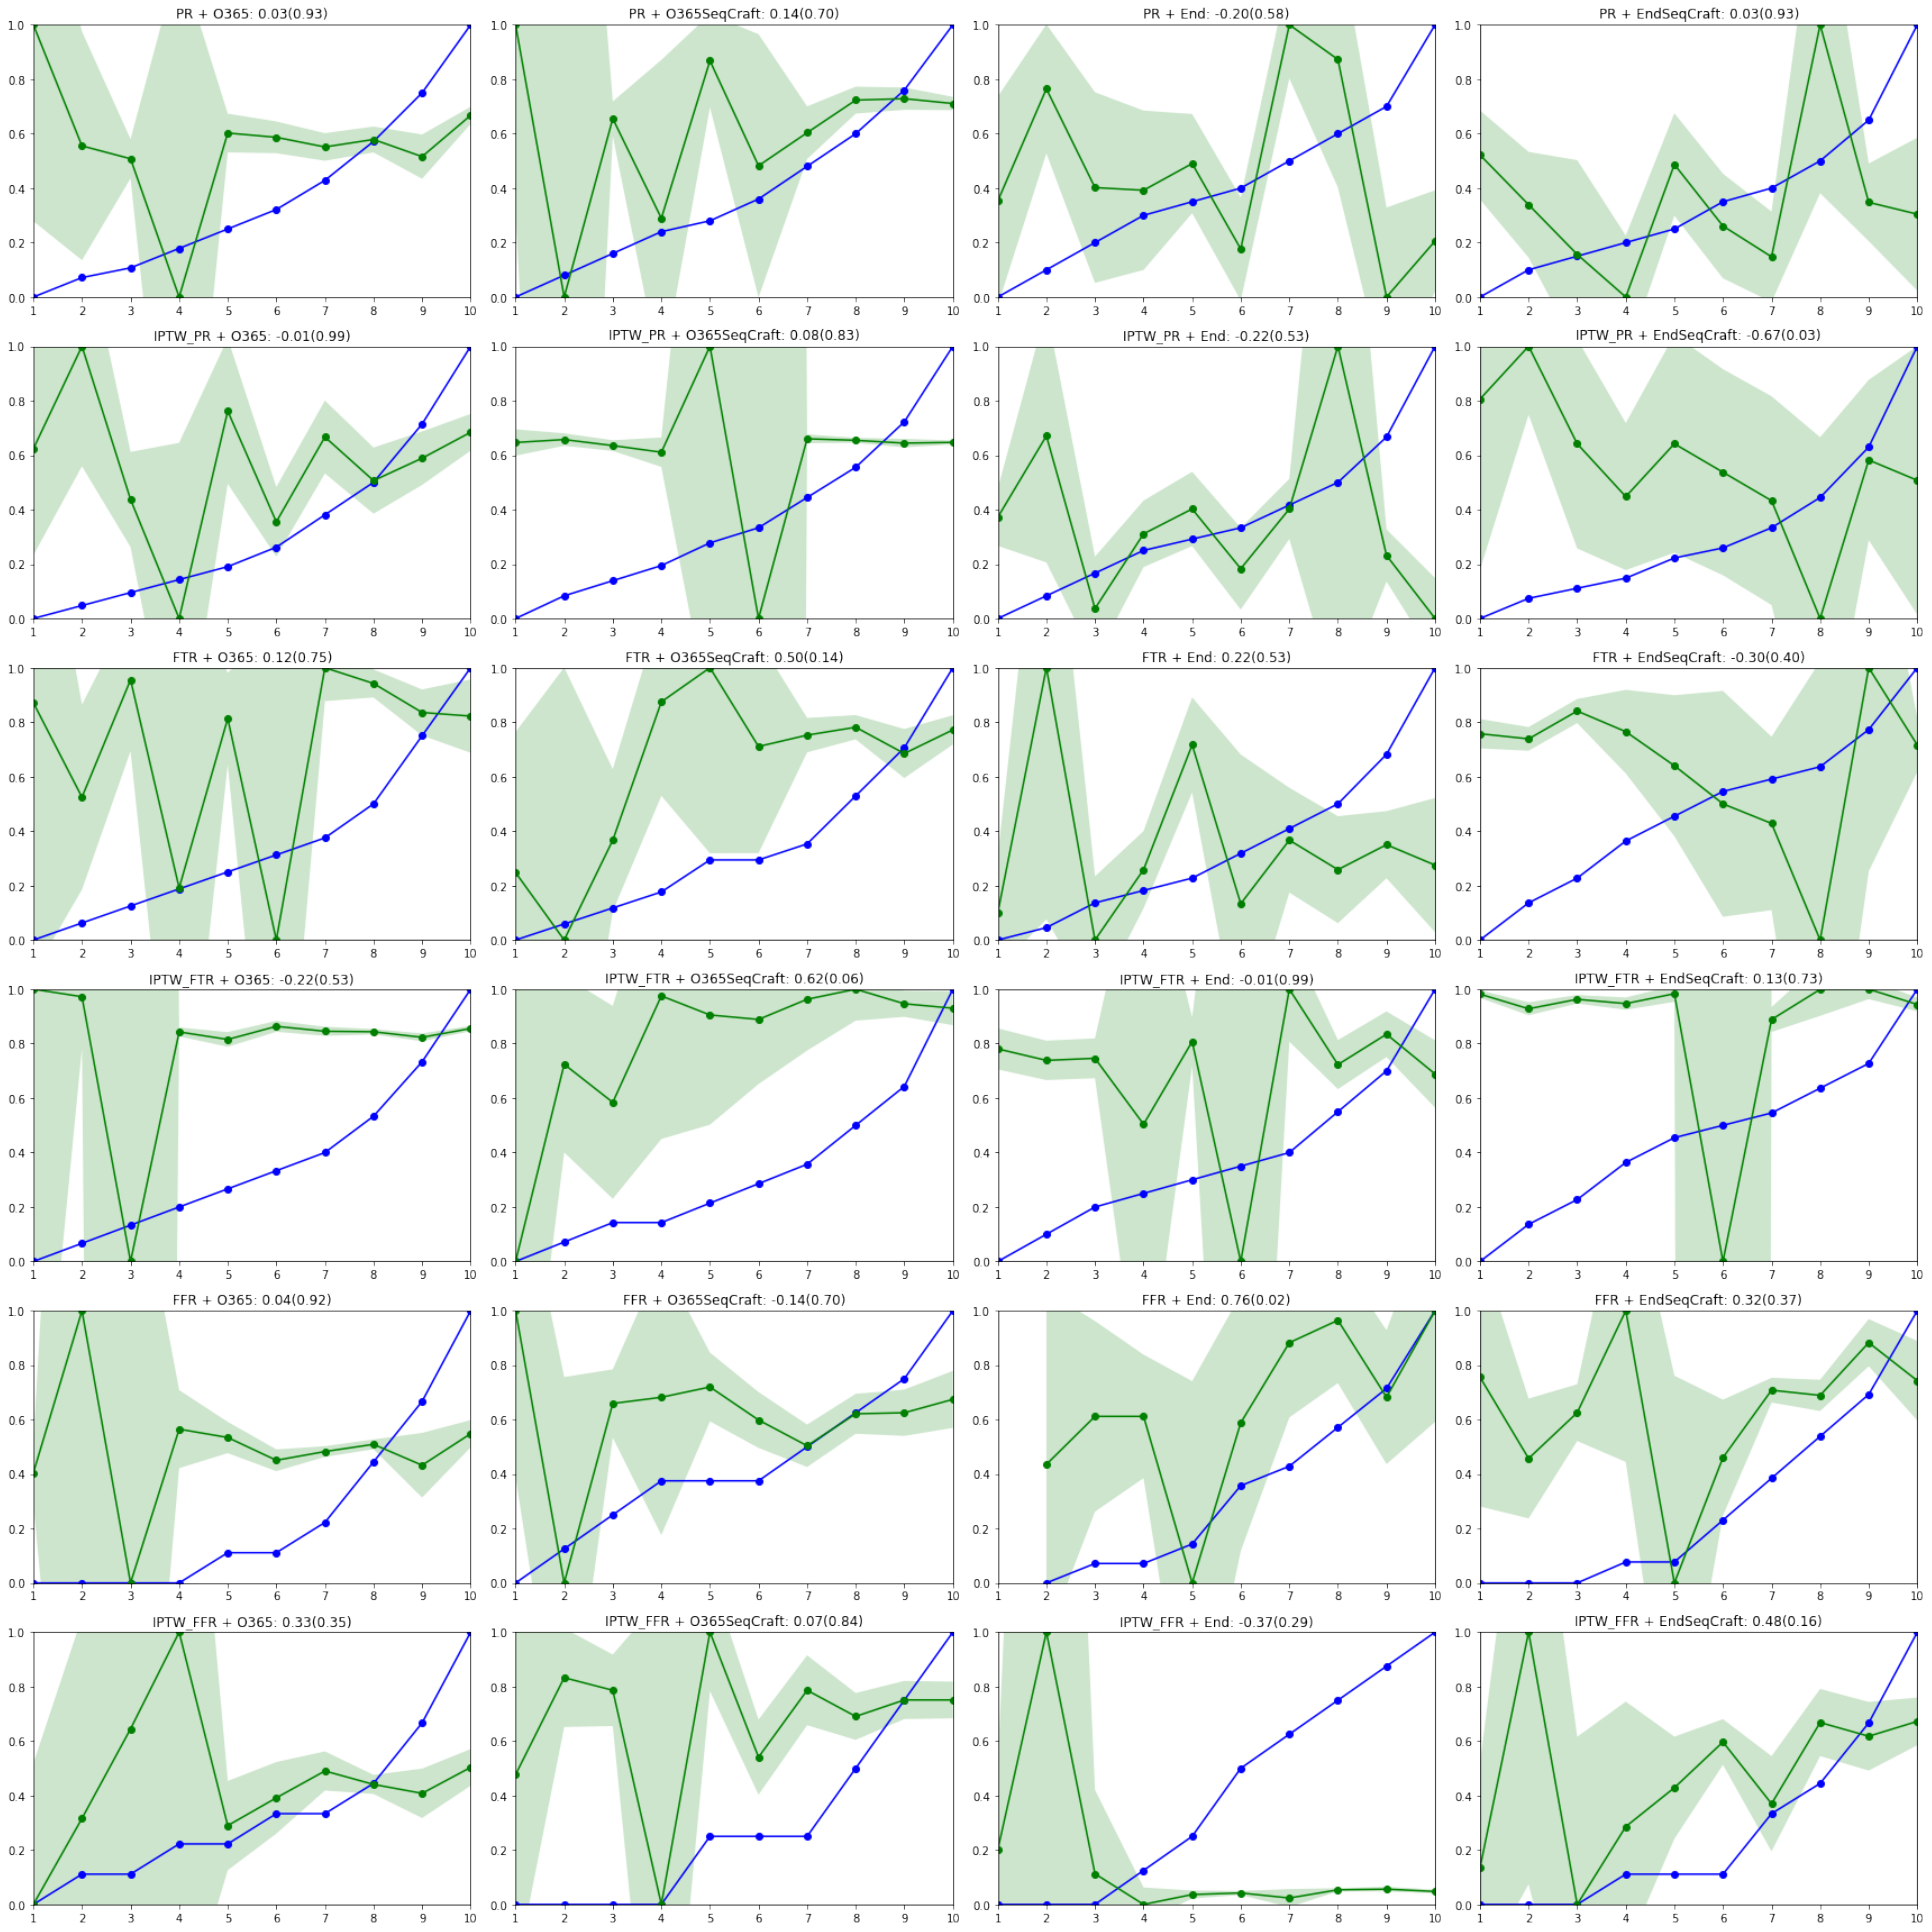}
%     \caption{ITE evaluation (ML models)}
% \end{figure*}

% \begin{figure*}
%     \centering
%     \includegraphics[width= \textwidth]{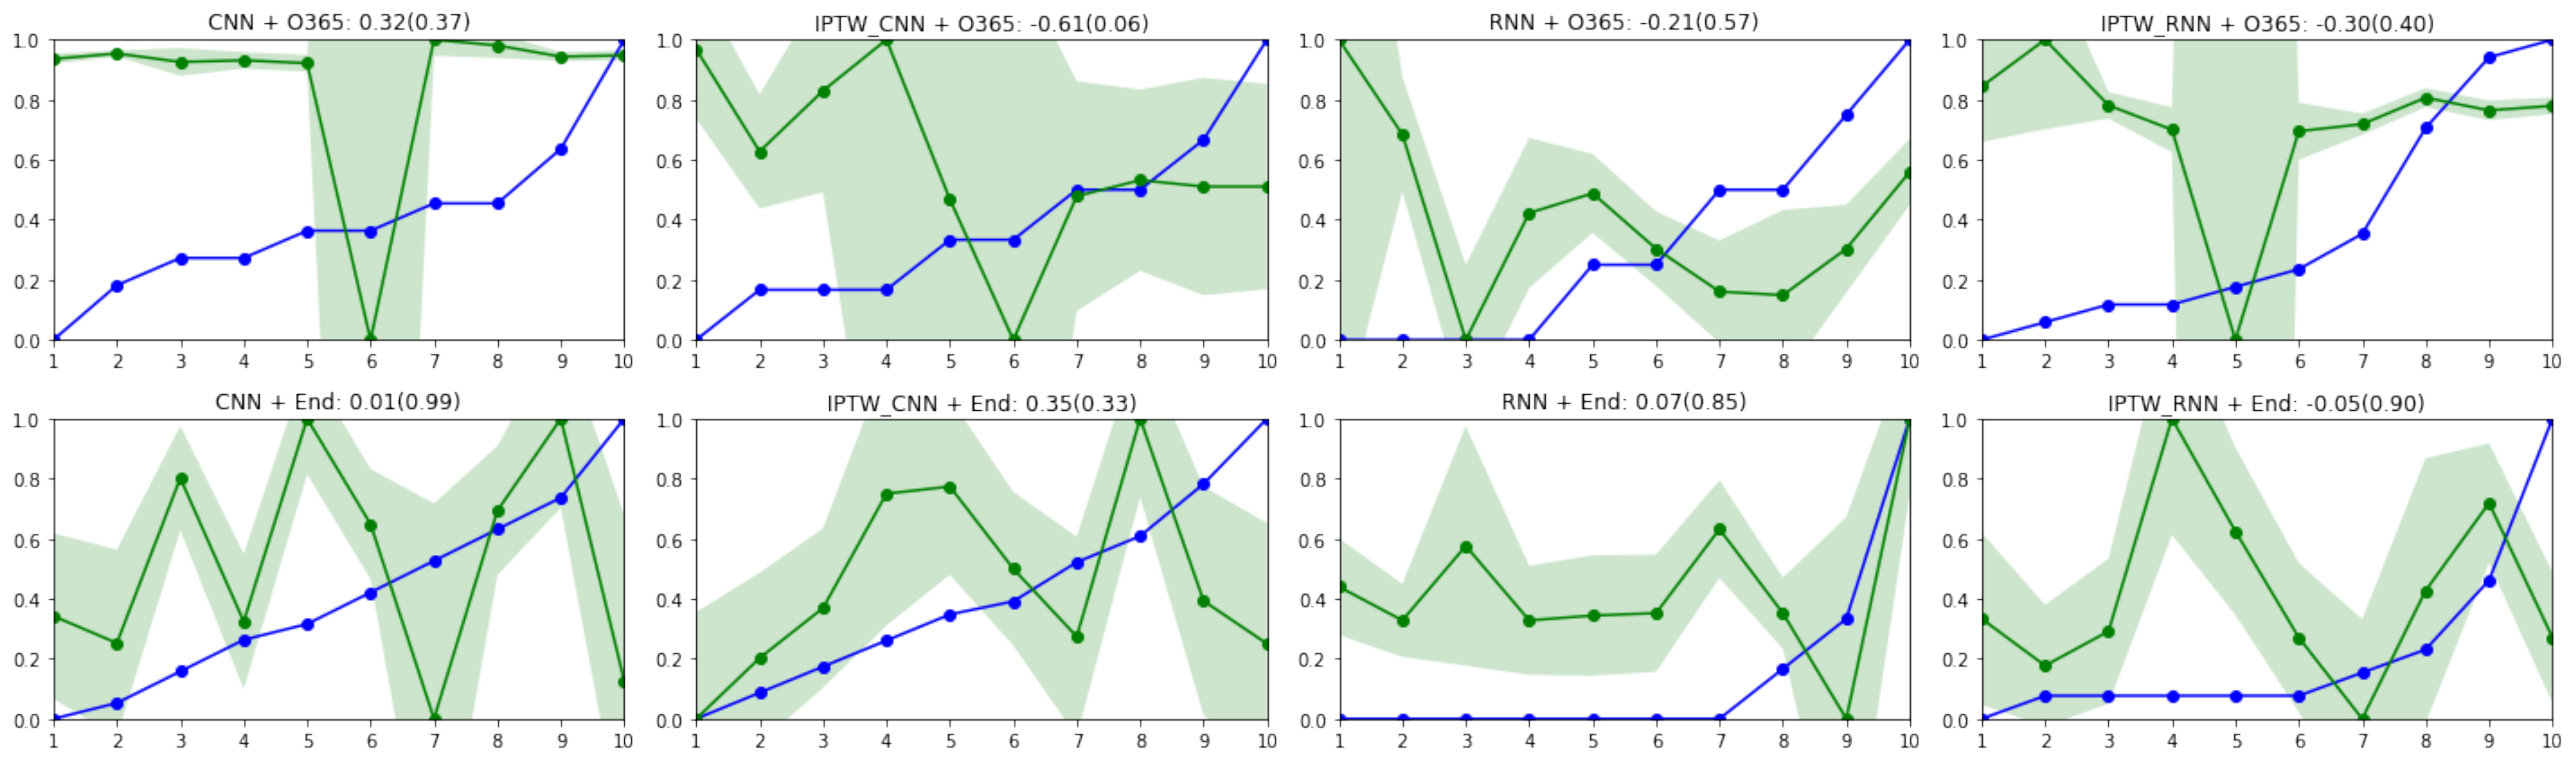}
%     \caption{ITE evaluation (DL models)}
% \end{figure*}

% \begin{figure*}
%     \centering
%     \includegraphics[width= \textwidth]{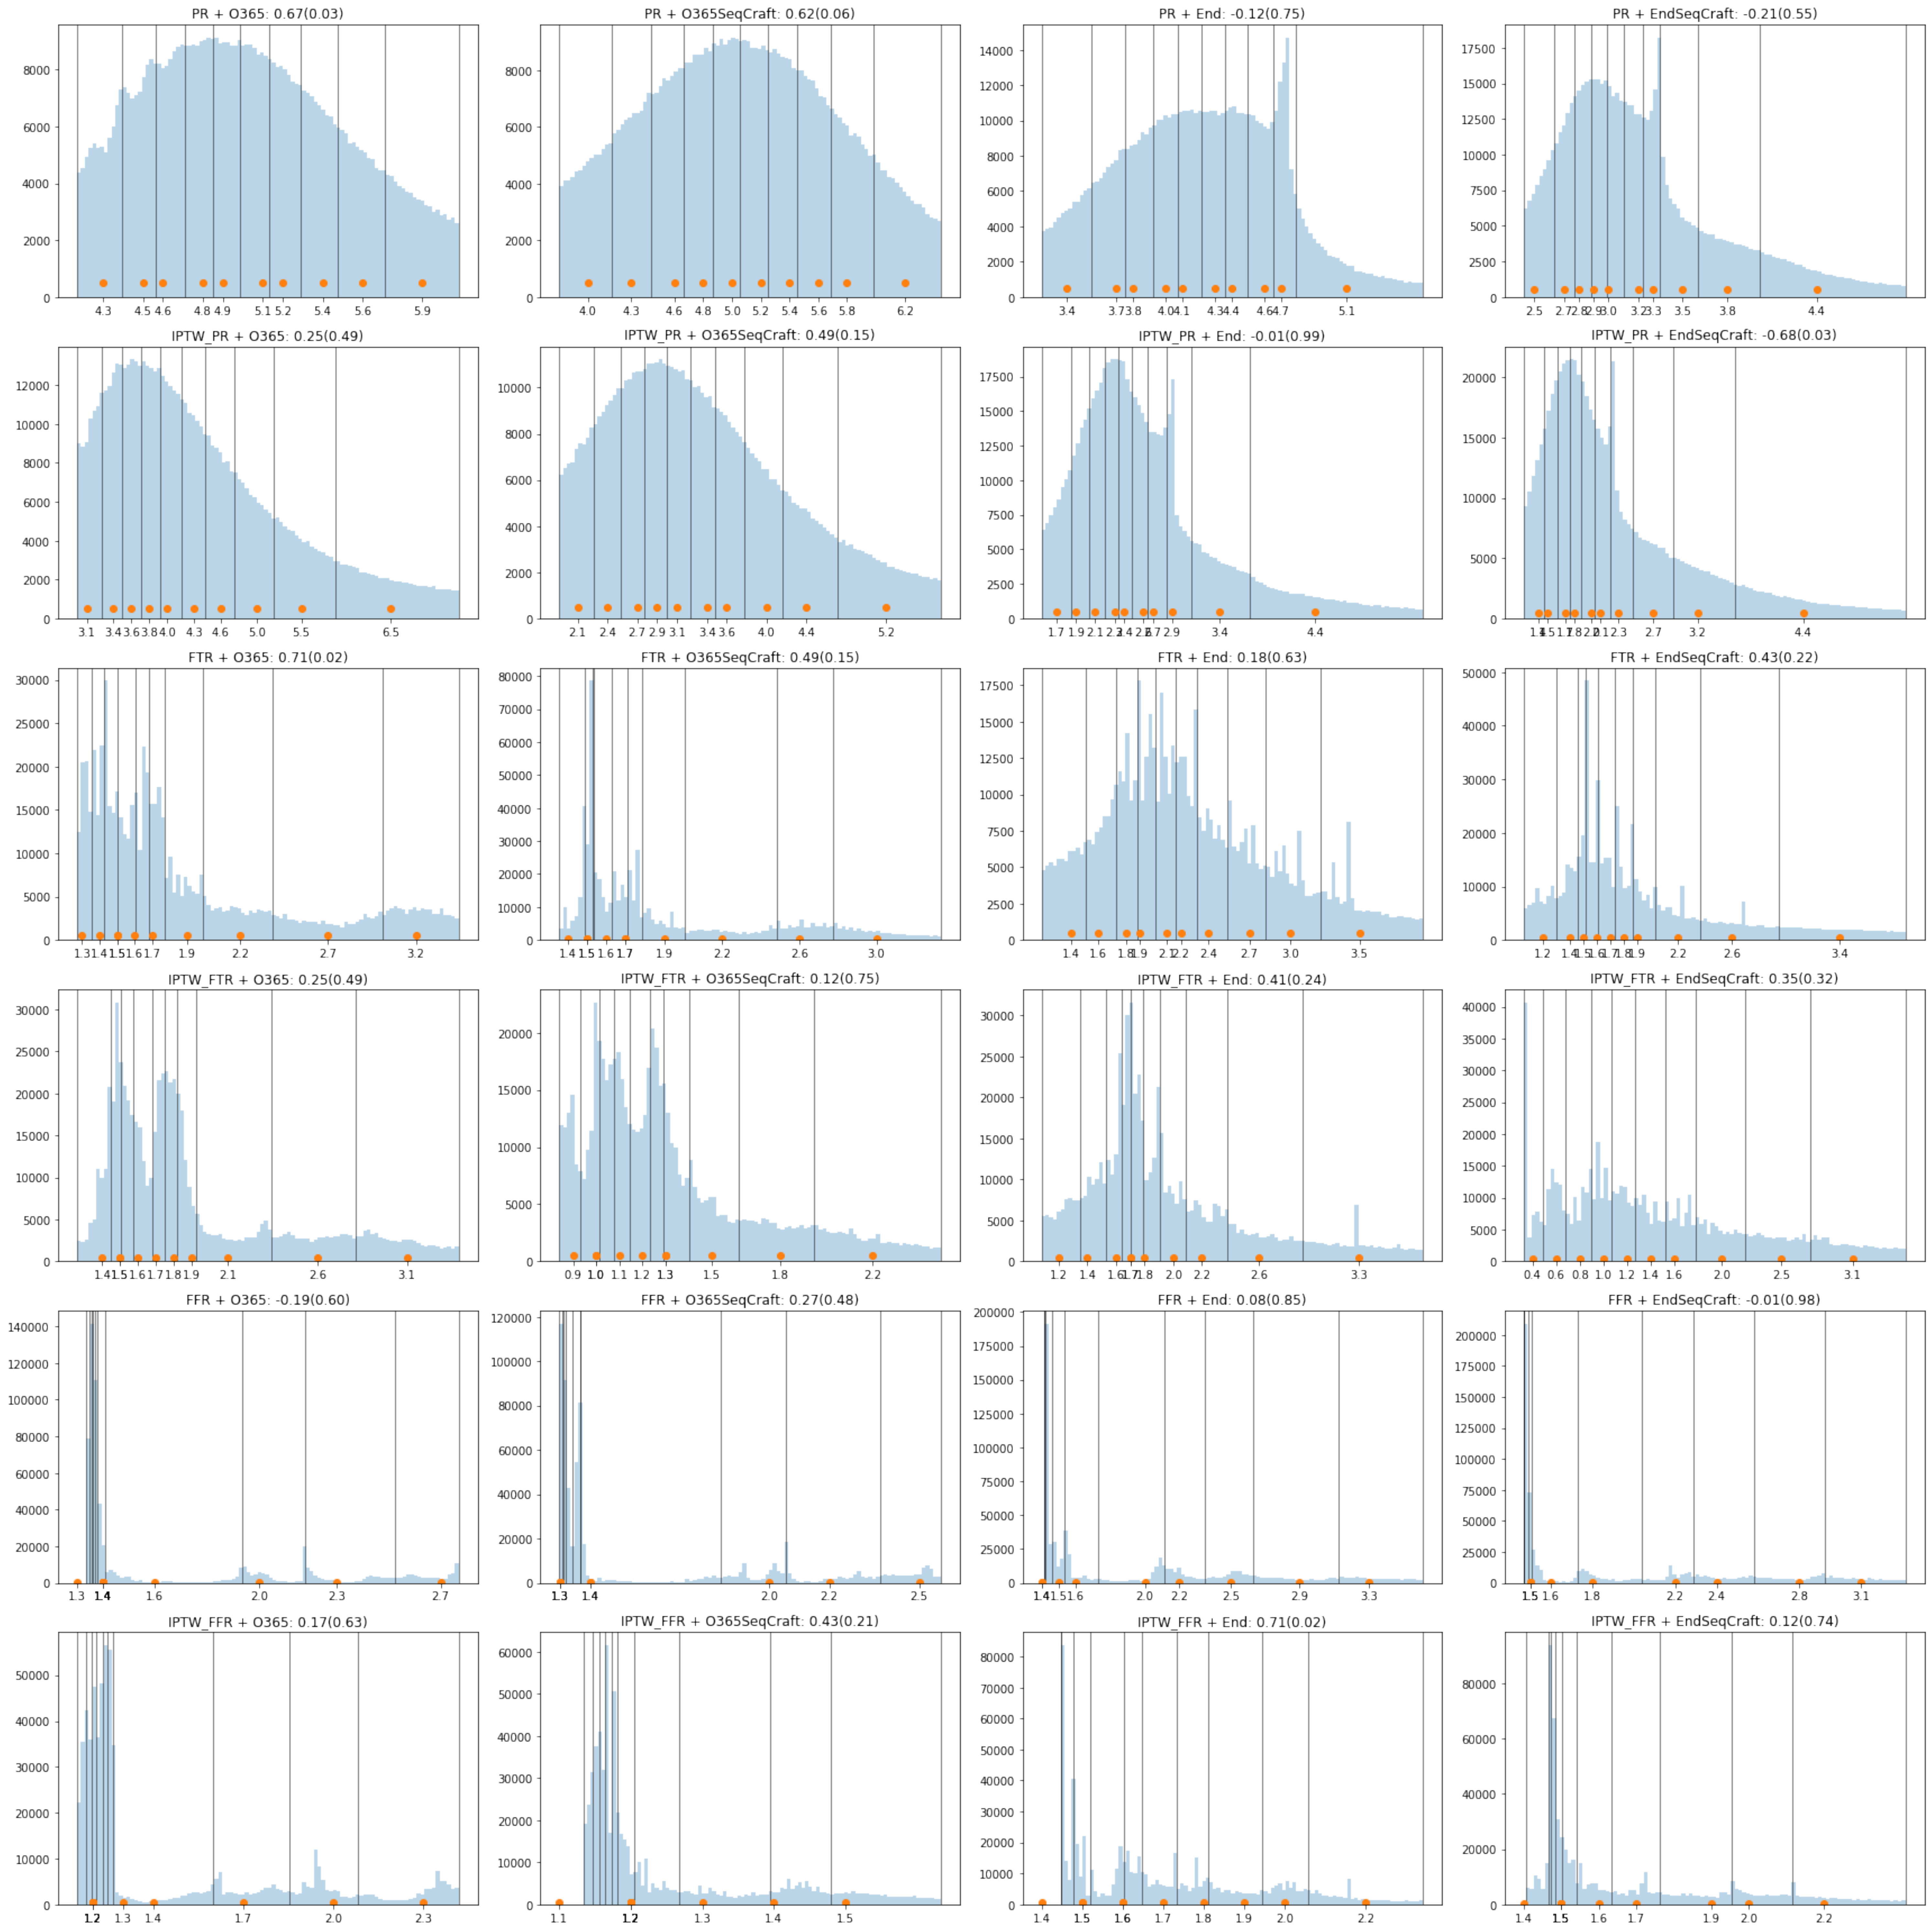}
%     \caption{ITE distribution (ML models)}
% \end{figure*}
